# Supplementary material for: Building Machine Translation Systems for the Next Thousand Languages
Source: arXiv:2205.03983 source file (2022-07-06)
Supplement: Supplementary file 1 [file table_unmterrors_appendix.tex]

\begin{table}[!htb]
\scriptsize % \tiny \scriptsize \footnotesize \small
      \centering
        \begin{tabular}{l p{0.47\linewidth} | p{0.44\linewidth}}
        sl & ``I believe that a \textbf{lion} is stronger than a \textbf{tiger}'' & ``there are more \textbf{tigers} in captivity than \textbf{sharks}'' \\
        \hline
ak & I believe that a \correct{lion} is stronger than a \mistake{leopard}. &  more \mistake{deer} have been caught in caves than in \mistake{dense water}. \\
% ay & The true captain of the \mistake{liwuna} is still chacmani and the \correct{tiger} is a cat. &  Many \mistake{otters} are closed and not \correct{sharks} \\
bho & In my opinion, a \correct{lion} is much stronger than a \correct{tiger}. &  There are more \mistake{lions} in captivity than \correct{sharks}. \\
bm & I believe that the \correct{lion} is stronger than the \mistake{lion's mane}. &  I do catch more \mistake{lion cubs} than \mistake{raccoons}. \\
doi & I believe that \mistake{seizures} are more severe than \mistake{epilepsy}. &  More \mistake{seals} are in captivity than \correct{sharks}. \\
dv & I believe a \correct{lion} would be stronger than a \mistake{miniature crocodile}. &  There are more \correct{miniature crocodiles} in captivity than \correct{sharks}. \\
ee & I am convinced that a \correct{lion} is stronger than a \mistake{wolf}. &  some \mistake{sheep} are in prison more than \correct{wolves}. \\
ff & I think a \mistake{rabbit} is stronger than a \mistake{squirrel}. &  \mistake{cewnguuji} is more common in \mistake{tiwaande} and rekee. \\
gn & I believe that the \correct{lion} is stronger than the \mistake{jackal}. &  there are more in the \mistake{jackal} pen than in the \mistake{fish}. \\
gom & I believe that a \correct{lion} is stronger than a \correct{tiger}. &  More \correct{tigers} have been captured than \mistake{peacocks}. \\
ilo & I believe a \correct{lion} is stronger than a \correct{tiger}. &  there are more \correct{tigers} in captivity than \correct{sharks}. \\
kl & I think the \correct{lion} is more violent than the \correct{tiger}. &  More \correct{tigers} than \mistake{eagles} are in the wild. \\
kri & I believe in forcing a \correct{lion}'s throne rather than a \correct{tiger}. &  more \correct{tigers} have been captured than \correct{sharks}. \\
lus & I think the \correct{lion} is stronger than the \correct{tiger}. &  There are more \correct{tigers} than \correct{sharks}. \\
mai & I believe that \correct{lions} are stronger than \correct{tigers}. &  There were more \correct{tigers} in captivity than \mistake{SAARC}. \\
mni & I believe a \correct{snake} is stronger than a \mistake{crocodile}. &  They catch more \mistake{cats} than \correct{sharks}. \\
nso & I believe that a \correct{lion} is stronger than a \correct{tiger}. &  There are more \correct{tigers} to catch than \correct{sharks}. \\
om & I believe that a \correct{lion} is stronger than a \mistake{young man}. &  There are more \mistake{sharks} than \correct{sharks}. \\
% pcm & I believe a \correct{lion} is stronger than a \correct{tiger}. &  \correct{tigers} caught out of the bush are more numerous than \correct{sharks}. \\
qu & Is the \correct{lion} stronger than the \correct{tiger} &  There are more \correct{tigers} in Ch'achana than in \mistake{Tinurunquna} \\
sa & I believe that a \correct{lion} is stronger than a \correct{tiger}. &  There are more \correct{tigers} of captivity than \mistake{crocodiles}. \\
ti & I believe that a \correct{lion} is stronger than a \correct{tiger}. &  There are many more captured \correct{tigers} than \correct{sharks}. \\
ts & i believe the \correct{lion} is stronger than the \correct{tiger} &  \correct{tigers} are more confined than \mistake{squirrels} \\
yua & it seems to me a \mistake{chakmo'ole} is more powerful than an \mistake{elephant} &  more \mistake{red prisoners} than \correct{sharks}. \\
yue & I believe \correct{lions} are stronger than \correct{tigers}. &  More stranded \correct{tigers} than \correct{sharks}. \\
\hline
        \end{tabular}
        
    % % \caption{Translations of the sentence meaning "I believe that a lion is stronger than a tiger" from various languages into English. Those above the dashed line get these two nouns correct; those below substitute other animal names in.}
% % \label{tab:unmt_mistakes_lion}
\caption{Translations from various languages for the sentence meaning ``there are more tigers in captivity than sharks.'' This sentence exhibited among the most errors of any that we looked at. The word ``lion'' is correct X/Y times ... TODO Note that the mistranslations from the same language are often inconsistent, though \textit{tigers} is translated as \textit{miniature crocodiles} both times from Dhivehi. TODO organize in some noce way}
\label{tab:unmt_mistakes_sharks}
\end{table}

\begin{table*}
\scriptsize % \tiny \scriptsize \footnotesize \small
      \centering
        \begin{tabular}{l p{0.45\linewidth} | p{0.45\linewidth}}
\hline
\hline
sl & ``the first three colors are \textbf{red}, \textbf{orange}, and \textbf{yellow}'' & ``this is why \textbf{hair} turns \textbf{grey} with age.''      \\
\hline
ak & the first three colors are \correct{red}, \mistake{blue}, and \mistake{orange}. & this is why \correct{hair} turns \mistake{discolored} after a few years. \\
as & These first three colors are \correct{red}, \correct{orange} and \correct{yellow}. & This is why \correct{hair} turns \mistake{smoky} with age. \\
% ay & the first three colors are \correct{red}, \mistake{purple}, and \correct{yellow} & Therefore the \correct{hair} \mistake{falls out} in a very old person \\
bho & The first three colors are \correct{red}, \correct{orange} and \correct{yellow}. & This is why the \correct{hair} starts to turn \mistake{white} with age. \\
bm & the three-primary colors are \correct{red}, \mistake{negro}, and \mistake{black}. & so the \correct{hair} fell \mistake{white}. \\
doi & The first three colors are \correct{red}, \correct{orange} and \correct{yellow}. & This is the reason why \correct{hair} becomes \mistake{sticky} with age. \\
dv & The first three colors are \correct{red}, \correct{orange} and \correct{yellow}. & This is why \correct{hair} turns \mistake{white} with age. \\
ee & the primary colors are \correct{red}, \mistake{purple} and \mistake{orange}. & that is why \mistake{they} beat \mistake{flour} when they grow up. \\
ff & the first three colors are \mistake{white}, \correct{orange}, and \mistake{green}. & that is why the \mistake{head} is \mistake{ranked in the manger}. \\
gn & the three colors are \correct{red}, \mistake{purple} and \mistake{blue}. & and therefore our \correct{hair} grows \mistake{white} in old age. \\
gom & The first three colors are \correct{red}, \correct{orange} and \correct{yellow}. & This causes \correct{hair} to \mistake{grow out} with age. \\
ilo & the first three colors are \correct{red}, \mistake{dalandan}, and \correct{yellow}. & this is the reason why \correct{hair} turns \correct{gray} as age increases. \\
kl & The first three colors are \mistake{blue}, \correct{orange} and \mistake{blue}. & That’s why \mistake{my nuts} are getting \mistake{brighter} with age. \\
kri & the first three colors are \correct{red}, \correct{orange}, and \correct{yellow}. & this is why \correct{hair} turns \correct{ash color} when old. \\
lus & The first three colors are \correct{red}, \mistake{purple} and \mistake{bright}. & This is why \correct{hair loss} occurs when we grow old. \\
mai & The first three colors are \correct{red}, \correct{orange} and \correct{yellow}. & Here is the reason why \correct{hair} turns \mistake{white} with age. \\
mni & The first three colors are \correct{red}, \mistake{yellow}, and \mistake{blue}. & That is why the \correct{hair} \mistake{changes color} with age. \\
nso & The first three colors are \correct{red}, \correct{orange} and \mistake{purple}. & That is why \correct{hair} turns \mistake{white} with age. \\
om & These three primary colors are:\correct{Red},\correct{Orange} and \correct{yellow}. & The \correct{hair} therefore becomes \mistake{dull} with age. \\
% pcm & the first three colors are \correct{red}, \correct{orange}, and \correct{yellow}. & this is why \correct{hair} changes to \correct{gray} color as a person ages. \\
qu & The first three colors are \correct{red}, \mistake{fire red}, and \correct{yellow}. & Over the years, the \correct{hair} turns \mistake{white} \\
sa & The first three colors are \correct{red}, \mistake{yellow} and \mistake{saffron}. & Therefore the \correct{hair} becomes \mistake{white} with increasing age. \\
ti & Those first three colors are \correct{red},\correct{orange} and \correct{yellow}. & This is why \correct{hair} turns to \correct{gray} with age. \\
ts & the first three colors are \correct{red}, \mistake{purple} and \mistake{pink} & because \correct{hair} turns \mistake{white} with age \\
yua & the first colors are \correct{red},\mistake{red} and \correct{yellow}. & therefore the \correct{hair} turns \correct{gray} as it gets older. \\
yue & The first three colors are \correct{red}, \correct{orange} and \correct{yellow}. & This is why \correct{hair} turns \mistake{white} with age. \\
\hline
\end{tabular}

\caption{Translations from various languages for the sentence meaning ``the first three colors are red, orange, and yellow'' and ``this is why hair turns grey with age'' into English. The models demonstrate typical difficulties with nouns that occur in similar distributional contexts, like colors.}
\label{tab:unmt_mistakes_colors}
\end{table*}
